# Supplementary material for: Neural Camera Models
Source: arXiv:2208.12903 source file (2022-08-27)
Supplement: Supplementary file 1 [file supp_mat.tex]

\section{Implementation Details}

\subsection{Training parameters}

We implemented our models using PyTorch,
% \footnote{Training and inference code will be made available upon publication.}, 
with distributed training across eight A100 GPUs. We used grid search to choose training parameters, that include: view synthesis weight $\lambda_s = 5.0$, virtual camera loss weight $\lambda_v=0.5$, virtual camera projection noise $\sigma_v = 0.25$, canonical jittering noise $\sigma_t=\sigma_r=0.1$, and batch size $b=32$ ($4$ per GPU). We use the AdamW optimizer~\cite{loshchilov2019decoupled}, with standard parameters $\beta_1=0.9$, $\beta_2=0.999$, a weight decay of $w=10^{-4}$, and an initial learning rate of $lr=2 \cdot 10^{-4}$. For our stereo experiments, we train for $200$ epochs, halving the learning rate every $80$ epochs. For our video experiments, we train for $100$ epochs, halving the learning rate every $40$ epochs. Higher-resolution fine-tuning is performed for $50$ epochs for stereo experiments, and $10$ epochs for video experiments, with $lr=2 \cdot 10^{-5}$.

\subsection{Architecture Details}

Following recent work~\cite{yifan2021input}, we use $K_o=20$ and $K_r=10$ as the number of Fourier frequencies for camera embeddings, with maximum resolution $\mu_o = \mu_r = 60$. Our encoder embeddings have dimensionality $C_e=960 + 186 = 1146$, due to the use of both image and camera information. Our decoder embeddings have dimensionality $C_d=186$, since only camera information is required to produce estimates. Our latent representation $\mathcal{R}$ is of dimensionality $2048 \times 512$. Input images are resized to $128 \times 192$, and following standard protocol~\cite{deepv2d} output depth maps are compared to ground-truth resized to $480 \times 640$. We use the following hyperparameters for our Perceiver~IO implementation: $1$ block, $1$ input cross-attention, $8$ self-attention layers (with $8$ heads) and $1$ output cross-attention.  Cross attention layers have only $1$ head. We found that larger Perceiver~IO models (i.e., with more blocks, number of heads, and self-/cross-attention layers) did not improve results and significantly increased training time. The latest developments in the Perceiver architecture~\cite{hier-perceiver} could be used to further improve performance and inference speed, and will be considered in future work.

\section{Canonical Jittering Test-time Ablation}

In Section 4.3 of the main text, we ablate the effects of using our proposed data augmentation techniques, designed to improve multi-view consistency in the learned latent representation. In Figure 4b we provide an additional experiment in which we vary the amount of virtual camera noise $\sigma_v$ at train and test time, and show that training at higher noise levels not only improves depth estimation performance at the target location (up to a certain value, of $\sigma_v=0.25$m), but also when decoding estimates from novel viewpoints. 

Here we perform a similar experiment targeting another proposed data augmentation technique: canonical jittering. Two different models were trained, with and without canonical jittering, and both were evaluated under different noise levels at test time.  Note that, while this augmentation does not change scene geometry, it changes the camera embeddings used for encoding and decoding information.
Results are presented in Table \ref{table:pose_jittering}. As we can see, the model trained with canonical jittering not only performs better when evaluating at the target location, but is also more robust to increasing levels of noise at test time. 
\captionsetup[table]{skip=6pt}
\begin{table}[t!]

\centering
{
\small
\setlength{\tabcolsep}{0.3em}
\begin{tabular}{|l|cccc|}
\toprule
\diagbox{Train}{Test} & 
$0.0$m  & 
$0.1$m &
$0.2$m &
$0.5$m
\\
\midrule
$0.0$m
&
$0.101$ & $0.202$ & $0.226$ & $0.291$ \\
$0.1$m
&
$0.097$ & $0.160$ & $0.184$ & $0.242$ \\ 
\bottomrule
\end{tabular}
}
\caption{\textbf{Effects of canonical jittering at train and test time}. The model trained with canonical jittering ($\sigma_t = \sigma_r = 0.1$m) not only performs better when evaluated at the target location ($\sigma_t = \sigma_r = 0.0$m), but is also more robust to different levels of canonical jittering at test time. The results shown are average Abs. Rel. of the two predicted stereo depths maps, without ground-truth scaling.}
%\vspace{-6mm}
\label{table:pose_jittering}
\end{table}

% Do we replicate information about the encoder here?

\section{Higher Resolution Fine-Tuning}
One of the main challenges of training Transformer-based architectures has been the $O(N^2)$ self-attention memory scaling with input size. 
This means that the resolution of recent models has been fairly limited (e.g. the view synthesis model of Sajjadi et al.~\cite{sajjadi2021scene} primarily trains on low-resolution images, with a highest resolution of $128 \times 176$), hindering their application to real-world scenes.  
Perceiver~IO decouples input resolution from the the learned latent representation, which enables training and real-time inference at higher resolutions~\cite{yifan2021input}.
In our experiments, we found it advantageous to train using a resolution curriculum, first at a lower resolution ($128 \times 192$), and then fine-tune at a higher resolution $(240 \times 320)$. Note that, because the camera parameters are also scaled to the proper resolution, the scene geometry does not change, only (a) the number of embeddings generated per camera, and (b) the image embeddings, since resolution changes image features.  Thus, training at lower resolutions enables the faster learning of our desired multi-view latent scene representation, which can then be fine-tuned at higher resolutions for further improvements.
As an alternative, we also experimented with the strategy of \textit{sampling} rays at higher resolution (similar to NeRF~\cite{mildenhall2020nerf} and SRT~\cite{sajjadi2021scene}). However, we found that this approach led to unstable training and longer convergence times. As future work, we plan to investigate how training and and inference can be scaled up to even higher resolutions. 

\begin{figure}[t!]
\captionsetup[subfloat]{labelformat=empty}
%%%%%%%%%%%%%%%%%%%%%%%%%%%%%%%%% 
\subfloat{\includegraphics[width=0.16\textwidth,height=1.4cm]{figures/files/iib_comparison/define/0000001682_rgb(0)_gt.png}} \!
\subfloat{\includegraphics[width=0.16\textwidth,height=1.4cm]{figures/files/iib_comparison/define/gt_1682.png}} \!
\subfloat{\includegraphics[width=0.17\textwidth,height=1.4cm]{figures/files/iib_comparison/define/pred_1682.png}}  \!
\subfloat{\includegraphics[width=0.17\textwidth,height=1.4cm]{figures/files/iib_comparison/define/diff_image_1682.png}} \! 
\subfloat{\includegraphics[width=0.16\textwidth,height=1.4cm]{figures/files/iib_comparison/iib/pred_1682.png}}  \!
\subfloat{\includegraphics[width=0.16\textwidth,height=1.4cm]{figures/files/iib_comparison/iib/diff_image_1682.png}}
\\
\subfloat{\includegraphics[width=0.16\textwidth,height=1.4cm]{figures/files/iib_comparison/define/0000000168_rgb(0)_gt.png}} \!
\subfloat{\includegraphics[width=0.16\textwidth,height=1.4cm]{figures/files/iib_comparison/define/gt_168.png}} \!
\subfloat{\includegraphics[width=0.17\textwidth,height=1.4cm]{figures/files/iib_comparison/define/pred_168.png}}  \!
\subfloat{\includegraphics[width=0.17\textwidth,height=1.4cm]{figures/files/iib_comparison/define/diff_image_168.png}} \!
\subfloat{\includegraphics[width=0.16\textwidth,height=1.4cm]{figures/files/iib_comparison/iib/pred_168.png}}  \!
\subfloat{\includegraphics[width=0.16\textwidth,height=1.4cm]{figures/files/iib_comparison/iib/diff_image_168.png}}
\\ 
\subfloat{\includegraphics[width=0.16\textwidth,height=1.4cm]{figures/files/iib_comparison/define/0000004754_rgb(0)_gt.png}} \!
\subfloat{\includegraphics[width=0.16\textwidth,height=1.4cm]{figures/files/iib_comparison/define/gt_4754.png}} \!
\subfloat{\includegraphics[width=0.17\textwidth,height=1.4cm]{figures/files/iib_comparison/define/pred_4754.png}}  \!
\subfloat{\includegraphics[width=0.17\textwidth,height=1.4cm]{figures/files/iib_comparison/define/diff_image_4754.png}}  \!
\subfloat{\includegraphics[width=0.16\textwidth,height=1.4cm]{figures/files/iib_comparison/iib/pred_4754.png}}  \!
\subfloat{\includegraphics[width=0.16\textwidth,height=1.4cm]{figures/files/iib_comparison/iib/diff_image_4754.png}}
\\ 
\subfloat[Input Image]{\includegraphics[width=0.16\textwidth,height=1.4cm]{figures/files/iib_comparison/define/0000001940_rgb(0)_gt.png}} \!
\subfloat[GT depth]{\includegraphics[width=0.16\textwidth,height=1.4cm]{figures/files/iib_comparison/define/gt_1940.png}} \!
\subfloat[DeFiNe depth]{\includegraphics[width=0.17\textwidth,height=1.4cm]{figures/files/iib_comparison/define/pred_1940.png}} \!
\subfloat[DeFiNe error]{\includegraphics[width=0.17\textwidth,height=1.4cm]{figures/files/iib_comparison/define/diff_image_1940.png}} \!
\subfloat[IIB depth]{\includegraphics[width=0.16\textwidth,height=1.4cm]{figures/files/iib_comparison/iib/pred_1940.png}} \!
\subfloat[IIB error]{\includegraphics[width=0.16\textwidth,height=1.4cm]{figures/files/iib_comparison/iib/diff_image_1940.png}}
%%%%%%%%%%%%%%%%%%%%%%%%%%%%%%%%%%%%%%%%%%%%%%%%
\caption{\textbf{Qualitative comparison of DeFiNe} relative to the IIB~\cite{yifan2021input} baseline.  
Our architecture improves depth estimation quality in (i) smooth and textureless areas, (ii) far away regions, and (iii) image boundaries and depth discontinuities.
%The first column is the stereo pair, the second column is the DeFiNe prediction for the left camera and its error map, the next column is the IIB prediction and its error map, and final column is the GT depth map.
%Note that the depth errors for the IIB model around image boundaries and depth discontinuities.  
%Our DeFiNe architecture is able to correctly predict depth in these regions.
}
\label{fig:iib}
%\vspace{-5mm}
\end{figure}

%\section{Additional Qualitative Results}
\section{Comparison to IIB}
IIB~\cite{yifan2021input} is a recently proposed stereo depth estimation method that also uses a Perceiver~IO-based architecture.  Their major contribution is a geometrically-motivated epipolar inductive bias to encourage multi-view consistency. In Table 1 and Figure 4 of the main text, we show that our DeFiNe architecture significantly improves over the IIB baseline on the ScanNet-Stereo benchmark ($0.116$ vs. $0.089$ Abs. Rel.).  
Given that code and pre-trained models to replicate the IIB results are not available, we trained a model following the instructions in~\cite{yifan2021input}, achieving similar performance as reported in the paper. 

Some qualitative examples from this model are depicted in Figure \ref{fig:iib}, as well as examples from our DeFiNe architecture. As we can see, our proposed 3D augmentations and joint view synthesis learning also lead to significant qualitative improvements over IIB results. In particular, we consistently perform better in smooth and textureless areas, as well as far away regions and depth discontinuities. We attribute this behavior to an increase in scene diversity due to our contributions, that enables the learning of a more consistent multi-view latent scene representation.

%DeFiNe and color decoding lead to significant improvements over IIB both quantitatively and qualitatively, using no epipolar constraints.  Note that depth errors both around depth discontinuities and around image boundaries are smaller for DeFiNe than for IIB, we hypothesize that this is the effect of 3D augmentations which provide a richer, more multi-view consistent scene representation.

% \section{Scene Representation Ablations}
% DeFiNe learns a scene representation from a sequence from images.  We provide a further ablation comparing the stereo results of DeFiNe to a monocular variant, mapping only the source image to the source depth map with the same architecture. This section text TBD results of monocular training with 3D augmentations.
% % maybe further evidence for 3D augmentation
% \include{tables/monocular_ablations}

\section{Depth from Novel Viewpoints}

In Table \ref{tab:intra_extra} we provide numerical values to complement our depth interpolation and extrapolation experiments (Figures 7a and 7b from the main text). These experiments show that querying from our learned latent representation improves over the explicit projection of information from encoded views, while also enabling the estimation of dense depth maps from novel viewpoints. Similarly, in Figure \ref{fig:extra_additional} we provide additional qualitative examples of depth extrapolation to future timesteps, showing how DeFiNe can reconstruct unseen portions of the environment in a geometrically-consistent way.  

\begin{table*}[t!]
%\vspace{-4mm}

\centering
{
\small
\setlength{\tabcolsep}{0.3em}
\subfloat[Depth interpolation results.  
Frames at {[}$t-5,t+5${]} are encoded, and depth maps corresponding to camera locations at  {[}$t-4,\dots,t+4${]} are decoded.
%$
%$[t-5,t+5]$ 
]{
\begin{tabular}{l|ccccccccc}
\toprule
Timestep & $-4$ & $-3$ & $-2$ & $-1$ & $0$ & $+1$ & $+2$ & $+3$ & $+4$ \\
\midrule
\% valid pixels & $77.7$ & $68.5$ & $62.6$ & $59.5$ & $58.2$ & $58.7$ & $61.2$ & $66.6$ & $75.9$ \\
\toprule
Monodepth2~\cite{monodepth2} & 0.325 & 0.336 & 0.346 & 0.354 & 0.361 & 0.359 & 0.354 & 0.347 & 0.338 \\
PackNet~\cite{packnet}    & 0.305 & 0.318 & 0.330 & 0.341 & 0.344 & 0.344 & 0.336 & 0.327 & 0.338 \\
BTS~\cite{lee2019big}        & 0.296 & 0.306 & 0.320 & 0.329 & 0.334 & 0.326 & 0.327 & 0.319 & 0.303 \\
\midrule
DeFiNe (projection) & 0.226 & 0.239 & 0.251 & 0.259 & 0.268 & 0.261 & 0.254 & 0.244 & 0.231 \\
DeFiNe (query)      & 0.222 & 0.230 & 0.237 & 0.240 & 0.242 & 0.246 & 0.245 & 0.240 & 0.231 \\
\midrule
\midrule
DeFiNe (query, all) & 0.361 & 0.381 & 0.398 & 0.408 & 0.412 & 0.413 & 0.406 & 0.390 & 0.369 \\
\bottomrule
\end{tabular}
} \\
\subfloat[Depth extrapolation results. 
Frames at {[}$t-5,\dots,t-1${]} are encoded, and depth maps corresponding to camera locations at {[}$t,\dots,t+8${]} are decoded.
]{
\begin{tabular}{l|ccccccccc}
\toprule
Timestep & $0$ & $1$ & $2$ & $3$ & $4$ & $5$ & $6$ & $7$ & $8$ \\
\midrule
\% valid pixels & $91.0$ & $76.1$ & $64.5$ & $55.9$ & $49.6$ & $45.2$ & $42.0$ & $39.5$ & $36.0$ \\
\toprule
Monodepth2~\cite{monodepth2} & 0.351 & 0.386 & 0.398 & 0.405 & 0.412 & 0.420 & 0.431 & 0.441 & 0.453 \\
PackNet~\cite{packnet} & 0.327 & 0.358 & 0.378 & 0.391 & 0.400 & 0.406 & 0.420 & 0.428 & 0.436 \\
BTS~\cite{lee2019big} & 0.315 & 0.331 & 0.357 & 0.377 & 0.392 & 0.401 & 0.413 & 0.424 & 0.429 \\
\midrule
DeFiNe (projection) & 0.258 & 0.276 & 0.288 & 0.298 & 0.311 & 0.323 & 0.331 & 0.340 & 0.348 \\
DeFiNe (query) & 0.237 & 0.260 & 0.271 & 0.280 & 0.289 & 0.298 & 0.307 & 0.317 & 0.326 \\
\midrule
\midrule
DeFiNe (query, all) & 0.326 & 0.370 & 0.405 & 0.438 & 0.468 & 0.495 & 0.520 & 0.543 & 0.563 \\
\bottomrule
\end{tabular}
}
}
\caption{\textbf{Depth interpolation and extrapolation results}, on ScanNet (complementary to Figures 7a and 7b of the main text). On valid projected pixels, DeFiNe (query) outperforms the explicit projection of all considered single-frame baselines, and it also outperforms the explicit projection of its own estimates, obtained from encoded views (projection). Furthermore, it also enables the estimation of dense depth maps from novel viewpoints, which can be compared to the corresponding ground-truth from that location (query, all).} 
\label{tab:intra_extra}
%\vspace{-5mm}
\end{table*}

% \begin{table*}[t!]
% %\vspace{-4mm}
% \renewcommand{\arraystretch}{0.9}
% \centering
% {
% \small
% \setlength{\tabcolsep}{0.3em}

% }
% \caption{Depth extrapolation (Abs.\ Rel).} 
% \label{tab:extrapolation}
% \end{table*}

\begin{figure}[t!]
\captionsetup[subfloat]{labelformat=empty}
\vspace{2mm} \\ 
\rotatebox{90}{\hspace{1.0mm} \tiny{RGB}} \!
\subfloat{\includegraphics[width=0.1\textwidth,height=0.85cm]{depth_field_networks/figures/files/forecast/3033/0000003033_rgb(0)_gt.png}} \hspace{0.1mm}
\subfloat{\includegraphics[width=0.1\textwidth,height=0.85cm]{depth_field_networks/figures/files/forecast/3033/0000003033_rgb(1)_gt.png}} \hspace{0.1mm}
\subfloat{\includegraphics[width=0.1\textwidth,height=0.85cm]{depth_field_networks/figures/files/forecast/3033/0000003033_rgb(2)_gt.png}} \hspace{0.1mm}
\subfloat{\includegraphics[width=0.1\textwidth,height=0.85cm]{depth_field_networks/figures/files/forecast/3033/0000003033_rgb(3)_gt.png}} \hspace{0.1mm}
\subfloat{\includegraphics[width=0.1\textwidth,height=0.85cm]{depth_field_networks/figures/files/forecast/3033/0000003033_rgb(4)_gt.png}} \hspace{0.1mm}
\subfloat{\includegraphics[width=0.1\textwidth,height=0.85cm]{depth_field_networks/figures/files/forecast/3033/0000003033_rgb(5)_gt.png}} \hspace{0.1mm}
\subfloat{\includegraphics[width=0.1\textwidth,height=0.85cm]{depth_field_networks/figures/files/forecast/3033/0000003033_rgb(6)_gt.png}} \hspace{0.1mm}
\subfloat{\includegraphics[width=0.1\textwidth,height=0.85cm]{depth_field_networks/figures/files/forecast/3033/0000003033_rgb(7)_gt.png}} \hspace{0.1mm}
\subfloat{\includegraphics[width=0.1\textwidth,height=0.85cm]{depth_field_networks/figures/files/forecast/3033/0000003033_rgb(8)_gt.png}} 
\\ 
\rotatebox{90}{\hspace{1.0mm} \tiny{GT}} \!
\subfloat{\includegraphics[width=0.1\textwidth,height=0.85cm]{depth_field_networks/figures/files/forecast/3033/0000003033_depth(0)_gt_viz.png}} \hspace{0.1mm}
\subfloat{\includegraphics[width=0.1\textwidth,height=0.85cm]{depth_field_networks/figures/files/forecast/3033/0000003033_depth(1)_gt_viz.png}} \hspace{0.1mm}
\subfloat{\includegraphics[width=0.1\textwidth,height=0.85cm]{depth_field_networks/figures/files/forecast/3033/0000003033_depth(2)_gt_viz.png}} \hspace{0.1mm}
\subfloat{\includegraphics[width=0.1\textwidth,height=0.85cm]{depth_field_networks/figures/files/forecast/3033/0000003033_depth(3)_gt_viz.png}} \hspace{0.1mm}
\subfloat{\includegraphics[width=0.1\textwidth,height=0.85cm]{depth_field_networks/figures/files/forecast/3033/0000003033_depth(4)_gt_viz.png}} \hspace{0.1mm}
\subfloat{\includegraphics[width=0.1\textwidth,height=0.85cm]{depth_field_networks/figures/files/forecast/3033/0000003033_depth(5)_gt_viz.png}} \hspace{0.1mm}
\subfloat{\includegraphics[width=0.1\textwidth,height=0.85cm]{depth_field_networks/figures/files/forecast/3033/0000003033_depth(6)_gt_viz.png}} \hspace{0.1mm}
\subfloat{\includegraphics[width=0.1\textwidth,height=0.85cm]{depth_field_networks/figures/files/forecast/3033/0000003033_depth(7)_gt_viz.png}} \hspace{0.1mm}
\subfloat{\includegraphics[width=0.1\textwidth,height=0.85cm]{depth_field_networks/figures/files/forecast/3033/0000003033_depth(8)_gt_viz.png}} 
\\ 
\rotatebox{90}{\hspace{0.4mm} \tiny{Proj.}}
\subfloat{\includegraphics[width=0.1\textwidth,height=0.85cm]{depth_field_networks/figures/files/forecast/3033/0000003033_depth_valid_gt(0)_pred_viz.png}} \hspace{0.1mm}
\subfloat{\includegraphics[width=0.1\textwidth,height=0.85cm]{depth_field_networks/figures/files/forecast/3033/0000003033_depth_valid_gt(1)_pred_viz.png}} \hspace{0.1mm}
\subfloat{\includegraphics[width=0.1\textwidth,height=0.85cm]{depth_field_networks/figures/files/forecast/3033/0000003033_depth_valid_gt(2)_pred_viz.png}} \hspace{0.1mm}
\subfloat{\includegraphics[width=0.1\textwidth,height=0.85cm]{depth_field_networks/figures/files/forecast/3033/0000003033_depth_valid_gt(3)_pred_viz.png}} \hspace{0.1mm}
\subfloat{\includegraphics[width=0.1\textwidth,height=0.85cm]{depth_field_networks/figures/files/forecast/3033/0000003033_depth_valid_gt(4)_pred_viz.png}} \hspace{0.1mm}
\subfloat{\includegraphics[width=0.1\textwidth,height=0.85cm]{depth_field_networks/figures/files/forecast/3033/0000003033_depth_valid_gt(5)_pred_viz.png}} \hspace{0.1mm}
\subfloat{\includegraphics[width=0.1\textwidth,height=0.85cm]{depth_field_networks/figures/files/forecast/3033/0000003033_depth_valid_gt(6)_pred_viz.png}} \hspace{0.1mm}
\subfloat{\includegraphics[width=0.1\textwidth,height=0.85cm]{depth_field_networks/figures/files/forecast/3033/0000003033_depth_valid_gt(7)_pred_viz.png}} \hspace{0.1mm}
\subfloat{\includegraphics[width=0.1\textwidth,height=0.85cm]{depth_field_networks/figures/files/forecast/3033/0000003033_depth_valid_gt(8)_pred_viz.png}} 
\\ 
\rotatebox{90}{\hspace{0.1mm} \tiny{Pred.}} \!
\subfloat[$t$]{\includegraphics[width=0.1\textwidth,height=0.85cm]{depth_field_networks/figures/files/forecast/3033/0000003033_depth(0)_pred_viz.png}} \hspace{0.1mm}
\subfloat[$t+1$]{\includegraphics[width=0.1\textwidth,height=0.85cm]{depth_field_networks/figures/files/forecast/3033/0000003033_depth(1)_pred_viz.png}} \hspace{0.1mm}
\subfloat[$t+2$]{\includegraphics[width=0.1\textwidth,height=0.85cm]{depth_field_networks/figures/files/forecast/3033/0000003033_depth(2)_pred_viz.png}} \hspace{0.1mm}
\subfloat[$t+3$]{\includegraphics[width=0.1\textwidth,height=0.85cm]{depth_field_networks/figures/files/forecast/3033/0000003033_depth(3)_pred_viz.png}} \hspace{0.1mm}
\subfloat[$t+4$]{\includegraphics[width=0.1\textwidth,height=0.85cm]{depth_field_networks/figures/files/forecast/3033/0000003033_depth(4)_pred_viz.png}} \hspace{0.1mm}
\subfloat[$t+5$]{\includegraphics[width=0.1\textwidth,height=0.85cm]{depth_field_networks/figures/files/forecast/3033/0000003033_depth(5)_pred_viz.png}} \hspace{0.1mm}
\subfloat[$t+6$]{\includegraphics[width=0.1\textwidth,height=0.85cm]{depth_field_networks/figures/files/forecast/3033/0000003033_depth(6)_pred_viz.png}} \hspace{0.1mm}
\subfloat[$t+7$]{\includegraphics[width=0.1\textwidth,height=0.85cm]{depth_field_networks/figures/files/forecast/3033/0000003033_depth(7)_pred_viz.png}} \hspace{0.1mm}
\subfloat[$t+8$]{\includegraphics[width=0.1\textwidth,height=0.85cm]{depth_field_networks/figures/files/forecast/3033/0000003033_depth(8)_pred_viz.png}}
\vspace{2mm} \\ 
\rotatebox{90}{\hspace{1.0mm} \tiny{RGB}} \!
\subfloat{\includegraphics[width=0.1\textwidth,height=0.85cm]{depth_field_networks/figures/files/forecast/3017/0000003017_rgb(0)_gt.png}} \hspace{0.1mm}
\subfloat{\includegraphics[width=0.1\textwidth,height=0.85cm]{depth_field_networks/figures/files/forecast/3017/0000003017_rgb(1)_gt.png}} \hspace{0.1mm}
\subfloat{\includegraphics[width=0.1\textwidth,height=0.85cm]{depth_field_networks/figures/files/forecast/3017/0000003017_rgb(2)_gt.png}} \hspace{0.1mm}
\subfloat{\includegraphics[width=0.1\textwidth,height=0.85cm]{depth_field_networks/figures/files/forecast/3017/0000003017_rgb(3)_gt.png}} \hspace{0.1mm}
\subfloat{\includegraphics[width=0.1\textwidth,height=0.85cm]{depth_field_networks/figures/files/forecast/3017/0000003017_rgb(4)_gt.png}} \hspace{0.1mm}
\subfloat{\includegraphics[width=0.1\textwidth,height=0.85cm]{depth_field_networks/figures/files/forecast/3017/0000003017_rgb(5)_gt.png}} \hspace{0.1mm}
\subfloat{\includegraphics[width=0.1\textwidth,height=0.85cm]{depth_field_networks/figures/files/forecast/3017/0000003017_rgb(6)_gt.png}} \hspace{0.1mm}
\subfloat{\includegraphics[width=0.1\textwidth,height=0.85cm]{depth_field_networks/figures/files/forecast/3017/0000003017_rgb(7)_gt.png}} \hspace{0.1mm}
\subfloat{\includegraphics[width=0.1\textwidth,height=0.85cm]{depth_field_networks/figures/files/forecast/3017/0000003017_rgb(8)_gt.png}} 
\\ 
\rotatebox{90}{\hspace{1.0mm} \tiny{GT}} \!
\subfloat{\includegraphics[width=0.1\textwidth,height=0.85cm]{depth_field_networks/figures/files/forecast/3017/0000003017_depth(0)_gt_viz.png}} \hspace{0.1mm}
\subfloat{\includegraphics[width=0.1\textwidth,height=0.85cm]{depth_field_networks/figures/files/forecast/3017/0000003017_depth(1)_gt_viz.png}} \hspace{0.1mm}
\subfloat{\includegraphics[width=0.1\textwidth,height=0.85cm]{depth_field_networks/figures/files/forecast/3017/0000003017_depth(2)_gt_viz.png}} \hspace{0.1mm}
\subfloat{\includegraphics[width=0.1\textwidth,height=0.85cm]{depth_field_networks/figures/files/forecast/3017/0000003017_depth(3)_gt_viz.png}} \hspace{0.1mm}
\subfloat{\includegraphics[width=0.1\textwidth,height=0.85cm]{depth_field_networks/figures/files/forecast/3017/0000003017_depth(4)_gt_viz.png}} \hspace{0.1mm}
\subfloat{\includegraphics[width=0.1\textwidth,height=0.85cm]{depth_field_networks/figures/files/forecast/3017/0000003017_depth(5)_gt_viz.png}} \hspace{0.1mm}
\subfloat{\includegraphics[width=0.1\textwidth,height=0.85cm]{depth_field_networks/figures/files/forecast/3017/0000003017_depth(6)_gt_viz.png}} \hspace{0.1mm}
\subfloat{\includegraphics[width=0.1\textwidth,height=0.85cm]{depth_field_networks/figures/files/forecast/3017/0000003017_depth(7)_gt_viz.png}} \hspace{0.1mm}
\subfloat{\includegraphics[width=0.1\textwidth,height=0.85cm]{depth_field_networks/figures/files/forecast/3017/0000003017_depth(8)_gt_viz.png}} 
\\ 
\rotatebox{90}{\hspace{0.4mm} \tiny{Proj.}}
\subfloat{\includegraphics[width=0.1\textwidth,height=0.85cm]{depth_field_networks/figures/files/forecast/3017/0000003017_depth_valid_gt(0)_pred_viz.png}} \hspace{0.1mm}
\subfloat{\includegraphics[width=0.1\textwidth,height=0.85cm]{depth_field_networks/figures/files/forecast/3017/0000003017_depth_valid_gt(1)_pred_viz.png}} \hspace{0.1mm}
\subfloat{\includegraphics[width=0.1\textwidth,height=0.85cm]{depth_field_networks/figures/files/forecast/3017/0000003017_depth_valid_gt(2)_pred_viz.png}} \hspace{0.1mm}
\subfloat{\includegraphics[width=0.1\textwidth,height=0.85cm]{depth_field_networks/figures/files/forecast/3017/0000003017_depth_valid_gt(3)_pred_viz.png}} \hspace{0.1mm}
\subfloat{\includegraphics[width=0.1\textwidth,height=0.85cm]{depth_field_networks/figures/files/forecast/3017/0000003017_depth_valid_gt(4)_pred_viz.png}} \hspace{0.1mm}
\subfloat{\includegraphics[width=0.1\textwidth,height=0.85cm]{depth_field_networks/figures/files/forecast/3017/0000003017_depth_valid_gt(5)_pred_viz.png}} \hspace{0.1mm}
\subfloat{\includegraphics[width=0.1\textwidth,height=0.85cm]{depth_field_networks/figures/files/forecast/3017/0000003017_depth_valid_gt(6)_pred_viz.png}} \hspace{0.1mm}
\subfloat{\includegraphics[width=0.1\textwidth,height=0.85cm]{depth_field_networks/figures/files/forecast/3017/0000003017_depth_valid_gt(7)_pred_viz.png}} \hspace{0.1mm}
\subfloat{\includegraphics[width=0.1\textwidth,height=0.85cm]{depth_field_networks/figures/files/forecast/3017/0000003017_depth_valid_gt(8)_pred_viz.png}} 
\\ 
\rotatebox{90}{\hspace{0.1mm} \tiny{Pred.}} \!
\subfloat[$t$]{\includegraphics[width=0.1\textwidth,height=0.85cm]{depth_field_networks/figures/files/forecast/3017/0000003017_depth(0)_pred_viz.png}} \hspace{0.1mm}
\subfloat[$t+1$]{\includegraphics[width=0.1\textwidth,height=0.85cm]{depth_field_networks/figures/files/forecast/3017/0000003017_depth(1)_pred_viz.png}} \hspace{0.1mm}
\subfloat[$t+2$]{\includegraphics[width=0.1\textwidth,height=0.85cm]{depth_field_networks/figures/files/forecast/3017/0000003017_depth(2)_pred_viz.png}} \hspace{0.1mm}
\subfloat[$t+3$]{\includegraphics[width=0.1\textwidth,height=0.85cm]{depth_field_networks/figures/files/forecast/3017/0000003017_depth(3)_pred_viz.png}} \hspace{0.1mm}
\subfloat[$t+4$]{\includegraphics[width=0.1\textwidth,height=0.85cm]{depth_field_networks/figures/files/forecast/3017/0000003017_depth(4)_pred_viz.png}} \hspace{0.1mm}
\subfloat[$t+5$]{\includegraphics[width=0.1\textwidth,height=0.85cm]{depth_field_networks/figures/files/forecast/3017/0000003017_depth(5)_pred_viz.png}} \hspace{0.1mm}
\subfloat[$t+6$]{\includegraphics[width=0.1\textwidth,height=0.85cm]{depth_field_networks/figures/files/forecast/3017/0000003017_depth(6)_pred_viz.png}} \hspace{0.1mm}
\subfloat[$t+7$]{\includegraphics[width=0.1\textwidth,height=0.85cm]{depth_field_networks/figures/files/forecast/3017/0000003017_depth(7)_pred_viz.png}} \hspace{0.1mm}
\subfloat[$t+8$]{\includegraphics[width=0.1\textwidth,height=0.85cm]{depth_field_networks/figures/files/forecast/3017/0000003017_depth(8)_pred_viz.png}}
%%%%%%%%%%%%%%%%%%%%%%%%%%%%%%%%% 
\vspace{2mm} \\ 
\rotatebox{90}{\hspace{1.0mm} \tiny{RGB}} \!
\subfloat{\includegraphics[width=0.1\textwidth,height=0.85cm]{depth_field_networks/figures/files/forecast/1380/0000001380_rgb(0)_gt.png}} \hspace{0.1mm}
\subfloat{\includegraphics[width=0.1\textwidth,height=0.85cm]{depth_field_networks/figures/files/forecast/1380/0000001380_rgb(1)_gt.png}} \hspace{0.1mm}
\subfloat{\includegraphics[width=0.1\textwidth,height=0.85cm]{depth_field_networks/figures/files/forecast/1380/0000001380_rgb(2)_gt.png}} \hspace{0.1mm}
\subfloat{\includegraphics[width=0.1\textwidth,height=0.85cm]{depth_field_networks/figures/files/forecast/1380/0000001380_rgb(3)_gt.png}} \hspace{0.1mm}
\subfloat{\includegraphics[width=0.1\textwidth,height=0.85cm]{depth_field_networks/figures/files/forecast/1380/0000001380_rgb(4)_gt.png}} \hspace{0.1mm}
\subfloat{\includegraphics[width=0.1\textwidth,height=0.85cm]{depth_field_networks/figures/files/forecast/1380/0000001380_rgb(5)_gt.png}} \hspace{0.1mm}
\subfloat{\includegraphics[width=0.1\textwidth,height=0.85cm]{depth_field_networks/figures/files/forecast/1380/0000001380_rgb(6)_gt.png}} \hspace{0.1mm}
\subfloat{\includegraphics[width=0.1\textwidth,height=0.85cm]{depth_field_networks/figures/files/forecast/1380/0000001380_rgb(7)_gt.png}} \hspace{0.1mm}
\subfloat{\includegraphics[width=0.1\textwidth,height=0.85cm]{depth_field_networks/figures/files/forecast/1380/0000001380_rgb(8)_gt.png}} 
\\ 
\rotatebox{90}{\hspace{1.0mm} \tiny{GT}} \!
\subfloat{\includegraphics[width=0.1\textwidth,height=0.85cm]{depth_field_networks/figures/files/forecast/1380/0000001380_depth(0)_gt_viz.png}} \hspace{0.1mm}
\subfloat{\includegraphics[width=0.1\textwidth,height=0.85cm]{depth_field_networks/figures/files/forecast/1380/0000001380_depth(1)_gt_viz.png}} \hspace{0.1mm}
\subfloat{\includegraphics[width=0.1\textwidth,height=0.85cm]{depth_field_networks/figures/files/forecast/1380/0000001380_depth(2)_gt_viz.png}} \hspace{0.1mm}
\subfloat{\includegraphics[width=0.1\textwidth,height=0.85cm]{depth_field_networks/figures/files/forecast/1380/0000001380_depth(3)_gt_viz.png}} \hspace{0.1mm}
\subfloat{\includegraphics[width=0.1\textwidth,height=0.85cm]{depth_field_networks/figures/files/forecast/1380/0000001380_depth(4)_gt_viz.png}} \hspace{0.1mm}
\subfloat{\includegraphics[width=0.1\textwidth,height=0.85cm]{depth_field_networks/figures/files/forecast/1380/0000001380_depth(5)_gt_viz.png}} \hspace{0.1mm}
\subfloat{\includegraphics[width=0.1\textwidth,height=0.85cm]{depth_field_networks/figures/files/forecast/1380/0000001380_depth(6)_gt_viz.png}} \hspace{0.1mm}
\subfloat{\includegraphics[width=0.1\textwidth,height=0.85cm]{depth_field_networks/figures/files/forecast/1380/0000001380_depth(7)_gt_viz.png}} \hspace{0.1mm}
\subfloat{\includegraphics[width=0.1\textwidth,height=0.85cm]{depth_field_networks/figures/files/forecast/1380/0000001380_depth(8)_gt_viz.png}} 
\\ 
\rotatebox{90}{\hspace{0.4mm} \tiny{Proj.}}
\subfloat{\includegraphics[width=0.1\textwidth,height=0.85cm]{depth_field_networks/figures/files/forecast/1380/0000001380_depth_valid_gt(0)_pred_viz.png}} \hspace{0.1mm}
\subfloat{\includegraphics[width=0.1\textwidth,height=0.85cm]{depth_field_networks/figures/files/forecast/1380/0000001380_depth_valid_gt(1)_pred_viz.png}} \hspace{0.1mm}
\subfloat{\includegraphics[width=0.1\textwidth,height=0.85cm]{depth_field_networks/figures/files/forecast/1380/0000001380_depth_valid_gt(2)_pred_viz.png}} \hspace{0.1mm}
\subfloat{\includegraphics[width=0.1\textwidth,height=0.85cm]{depth_field_networks/figures/files/forecast/1380/0000001380_depth_valid_gt(3)_pred_viz.png}} \hspace{0.1mm}
\subfloat{\includegraphics[width=0.1\textwidth,height=0.85cm]{depth_field_networks/figures/files/forecast/1380/0000001380_depth_valid_gt(4)_pred_viz.png}} \hspace{0.1mm}
\subfloat{\includegraphics[width=0.1\textwidth,height=0.85cm]{depth_field_networks/figures/files/forecast/1380/0000001380_depth_valid_gt(5)_pred_viz.png}} \hspace{0.1mm}
\subfloat{\includegraphics[width=0.1\textwidth,height=0.85cm]{depth_field_networks/figures/files/forecast/1380/0000001380_depth_valid_gt(6)_pred_viz.png}} \hspace{0.1mm}
\subfloat{\includegraphics[width=0.1\textwidth,height=0.85cm]{depth_field_networks/figures/files/forecast/1380/0000001380_depth_valid_gt(7)_pred_viz.png}} \hspace{0.1mm}
\subfloat{\includegraphics[width=0.1\textwidth,height=0.85cm]{depth_field_networks/figures/files/forecast/1380/0000001380_depth_valid_gt(8)_pred_viz.png}} 
\\ 
\rotatebox{90}{\hspace{0.1mm} \tiny{Pred.}} \!
\subfloat[$t$]{\includegraphics[width=0.1\textwidth,height=0.85cm]{depth_field_networks/figures/files/forecast/1380/0000001380_depth(0)_pred_viz.png}} \hspace{0.1mm}
\subfloat[$t+1$]{\includegraphics[width=0.1\textwidth,height=0.85cm]{depth_field_networks/figures/files/forecast/1380/0000001380_depth(1)_pred_viz.png}} \hspace{0.1mm}
\subfloat[$t+2$]{\includegraphics[width=0.1\textwidth,height=0.85cm]{depth_field_networks/figures/files/forecast/1380/0000001380_depth(2)_pred_viz.png}} \hspace{0.1mm}
\subfloat[$t+3$]{\includegraphics[width=0.1\textwidth,height=0.85cm]{depth_field_networks/figures/files/forecast/1380/0000001380_depth(3)_pred_viz.png}} \hspace{0.1mm}
\subfloat[$t+4$]{\includegraphics[width=0.1\textwidth,height=0.85cm]{depth_field_networks/figures/files/forecast/1380/0000001380_depth(4)_pred_viz.png}} \hspace{0.1mm}
\subfloat[$t+5$]{\includegraphics[width=0.1\textwidth,height=0.85cm]{depth_field_networks/figures/files/forecast/1380/0000001380_depth(5)_pred_viz.png}} \hspace{0.1mm}
\subfloat[$t+6$]{\includegraphics[width=0.1\textwidth,height=0.85cm]{depth_field_networks/figures/files/forecast/1380/0000001380_depth(6)_pred_viz.png}} \hspace{0.1mm}
\subfloat[$t+7$]{\includegraphics[width=0.1\textwidth,height=0.85cm]{depth_field_networks/figures/files/forecast/1380/0000001380_depth(7)_pred_viz.png}} \hspace{0.1mm}
\subfloat[$t+8$]{\includegraphics[width=0.1\textwidth,height=0.85cm]{depth_field_networks/figures/files/forecast/1380/0000001380_depth(8)_pred_viz.png}}
%%%%%%%%%%%%%%%%%%%%%%%%%%%%%%%%%
\caption{\textbf{ScanNet depth extrapolation examples}, using DeFiNe. In each example, image and camera information from frames at $[t-5,\dots,t-1]$ is encoded, and depth maps corresponding to camera locations at $[t,\dots,t+8]$ are decoded, using only camera information. For each timestep, we show sparse projected ground-truth depth maps (third row), and dense predicted depth maps (fourth row). Our DeFiNe architecture is able to extrapolate from encoded information to fill in missing parts of the scene.}
\label{fig:extra_additional}
\end{figure}
